# Supplementary material for: Charge Asymmetry Suppresses Coarsening Dynamics in Polyelectrolyte Complex Coacervation
Source: arXiv:2308.16334 source file (2023-08-30)
Supplement: Supplementary file 1 [file spinodal_letter_SI.pdf]

# Supplementary Material for Charge Asymmetry Suppresses Coarsening Dynamics in Polyelectrolyte Complex Coacervation

Shensheng Chen and Zhen-Gang Wang*
*Division of Chemistry and Chemical Engineering, California Institute of Technology, Pasadena, CA 91125*

## A. Other simulation details

As per convention in DPD, the reduced number density is set to $\rho = 3.0$. The characteristic time scale is given by $\tau = \sqrt{mr_c^2/k_{\mathrm{B}}T}$. The integration time step is set to $\delta t = 0.05\tau$. To prepare 125 pairs in large systems for studying coarsening dynamics, we first equilibrate one pair with a given $\lambda$ in a $12r_c \times 12r_c \times 12r_c$ simulation box for $10^2\tau$, we then duplicate the small system 5 times in each direction to make the 125-pair systems in a $60r_c \times 60r_c \times 60r_c$ box. The positions and orientations of the polyion pairs become randomized on the order of $\sim 10\tau$, which is much shorter than the onset of coarsening ($> 100\tau$). The total simulation time is $5 \times 10^4\tau \sim 10^5\tau$. All the simulations are performed using the LAMMPS [1] platform.

## B. PMF calculation between two polyion pairs

We use the adaptive bias force (ABF) algorithm [2, 3]implemented in LAMMPS [4] to calculate the PMF between two polyion pairs in a simulation box of $24r_c \times 12r_c \times 12r_c$. The center of mass distance $r$ in the PMF calculation ranges from $0r_c$ to $15r_c$. The distance range is divided into consecutive windows of $0r_c \sim 1r_c$, $1r_c \sim 3r_c$, $3r_c \sim 6r_c$, $6r_c \sim 10r_c$ and $10r_c \sim 15r_c$ to improve the efficiency of the PMF calculations [3]. Each window is further divided into bins with equal width $0.1r_c$. The PMF in all windows reaches convergence before $5 \times 10^5\tau$.

## C. Polarization between two charge-balanced droplets

To study the polarization as two charge-balanced pairs approach each other, we calculate the electric dipole moment of each pair given by $\vec{P}_\alpha = \sum_i q_{\alpha,i}\vec{r}_{\alpha,i}$, where $q_{\alpha,i}$ is the charge on monomer $i$ and $r_{\alpha,i}$ is its vector position, and the sum is over all monomers in pair $\alpha$ ($\alpha = 1, 2$). The total dipole of the system is then $\vec{P} = \vec{P}_1 + \vec{P}_2$. $P_{||}$ is the projection of the total dipole moment onto the center-of-mass vector between the two pairs. Since by symmetry, $\langle P_{||}\rangle = 0$, we characterize the polarization by the second moment, $\langle P_{||}^2\rangle$.

In Fig. S1, we show $\langle P_{||}^2\rangle$ for three values of $\Delta a = 0, 10$, and 25. Polarization is stronger in systems with smaller $\Delta a$, with higher peak and wider range. Poorer solvent condition (larger $\Delta a$) results in weaker polarization, due to the compactness of the droplets.

[1] S. Plimpton, Fast Parallel Algorithms for Short-Range Molecular Dynamics, Journal of Computational Physics **117**, 1 (1995).
[2] E. Darve, D. Rodríguez-Gómez, and A. Pohorille, Adaptive biasing force method for scalar and vector free energy calculations, The Journal of Chemical Physics **128**, 144120 (2008).
[3] J. Comer, J. C. Gumbart, J. Hénin, T. Lelièvre, A. Pohorille, and C. Chipot, The Adaptive Biasing Force Method: Everything You Always Wanted To Know but Were Afraid To Ask, The Journal of Physical Chemistry B **119**, 1129 (2015).
[4] G. Fiorin, M. L. Klein, and J. Hénin, Using collective variables to drive molecular dynamics simulations, Molecular Physics **111**, 3345 (2013).

* zgw@caltech.edu

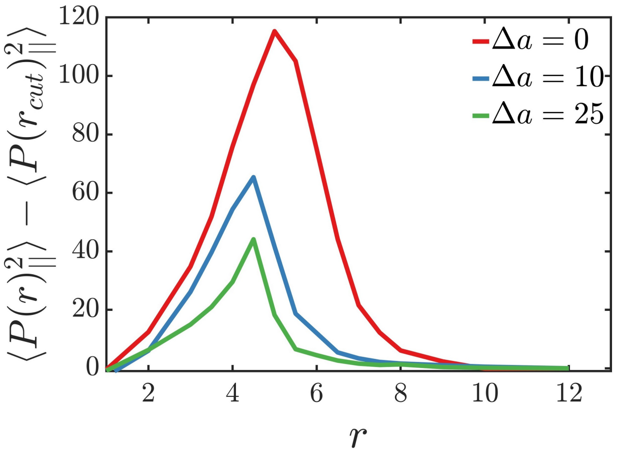


FIG. S1. Fluctuation of the longitudinal component of the polarization $\langle P^2_{||}\rangle$ as a function of the center-of-mass distance between the two polyion pairs under different solvent conditions. $r_{cut} = 12r_c$.
